# Supplementary material for: Vibronic fine structure in the nitrogen 1s photoelectron spectra from Franck-Condon simulations. III. Rules for amine/imine N atoms in small N-heterocycles
Source: arXiv:2311.06449 source file (2023-11-11)
Supplement: Supplementary file 1 [file SI-20231108.pdf]

# Supplementary Material for “Vibronic fine structure in the nitrogen 1s photoelectron spectra from Franck-Condon simulations. III. Rules for amine/imine N atoms in small N-heterocycles”

Minrui Wei,<sup>1</sup> Junxiang Zuo,<sup>1</sup> Guangjun Tian,<sup>2,\*</sup> and Weijie Hua<sup>1,†</sup>

<sup>1</sup>MIIT Key Laboratory of Semiconductor Microstructure and Quantum Sensing,  
Department of Applied Physics, School of Physics,  
Nanjing University of Science and Technology, 210094 Nanjing, China

<sup>2</sup>Key Laboratory for Microstructural Material Physics of Hebei Province,  
School of Science, Yanshan University, 066004 Qinhuangdao, China

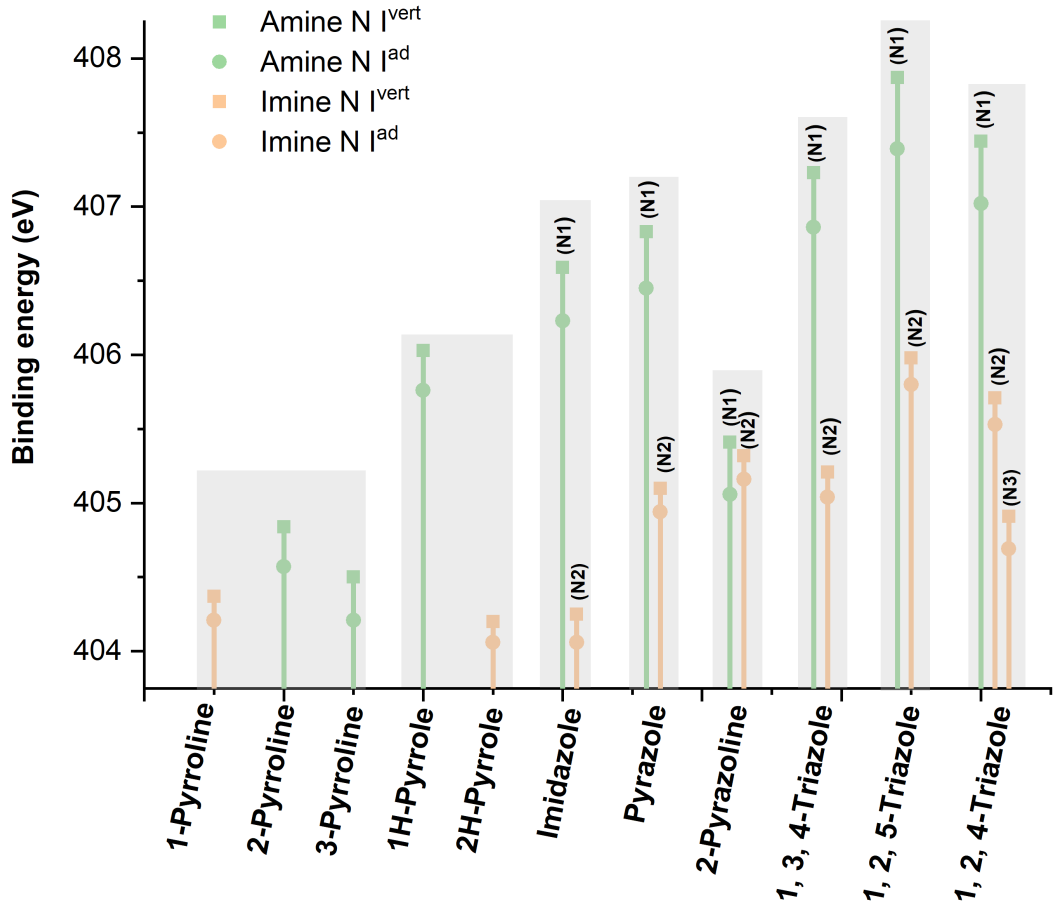

FIG. S1: Simulated vertical ( $I^{\text{vert}}$ ) and adiabatic ( $I^{\text{ad}}$ ) ionization potentials of 11 five-membered rings (this work) molecules. Rod tip shape differentiates between  $I^{\text{vert}}$  (square) and  $I^{\text{ad}}$  (circle) ionization potentials and the color differentiates between amine (orange) and imine (green) N atoms. Each gray area represents a group with the same molecular structure (or the same molecule).

\* tian@ysu.edu.cn

† wjhua@njust.edu.cn

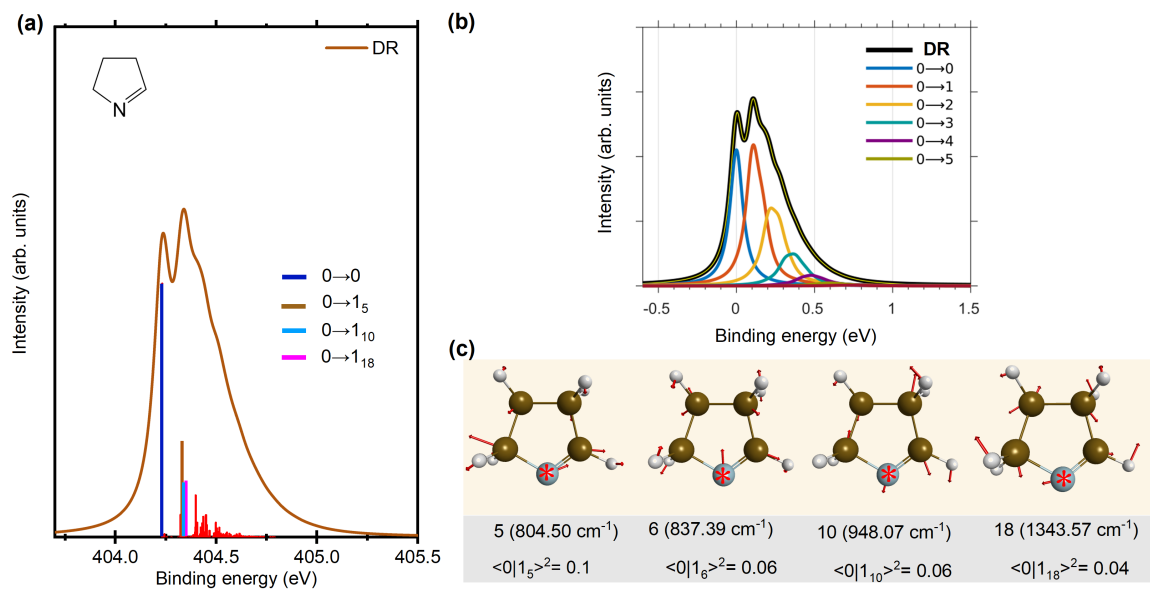

FIG. S2: (a) Simulated vibrationally-resolved N1s XPS spectrum of 1-pyrroline. (b) Analyses of contributions of different 0- $n$  transitions until convergence. 0-0 transition energy is taken as zero. (c) Active vibrational modes are identified in the final (FCH) state. For each mode, the mode index, frequency (in parentheses), and the FC factor are shown. Asterisk denotes the core ionization center.

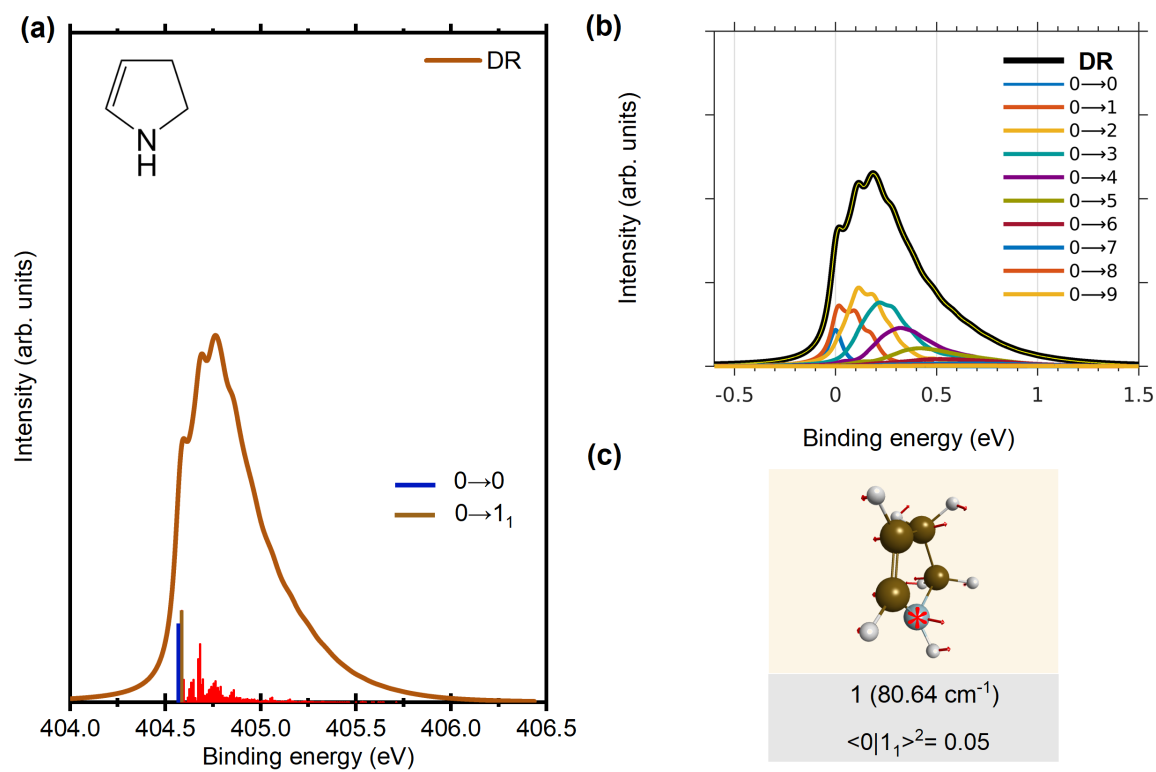

FIG. S3: The same as Fig. S2 for 2-pyrroline.

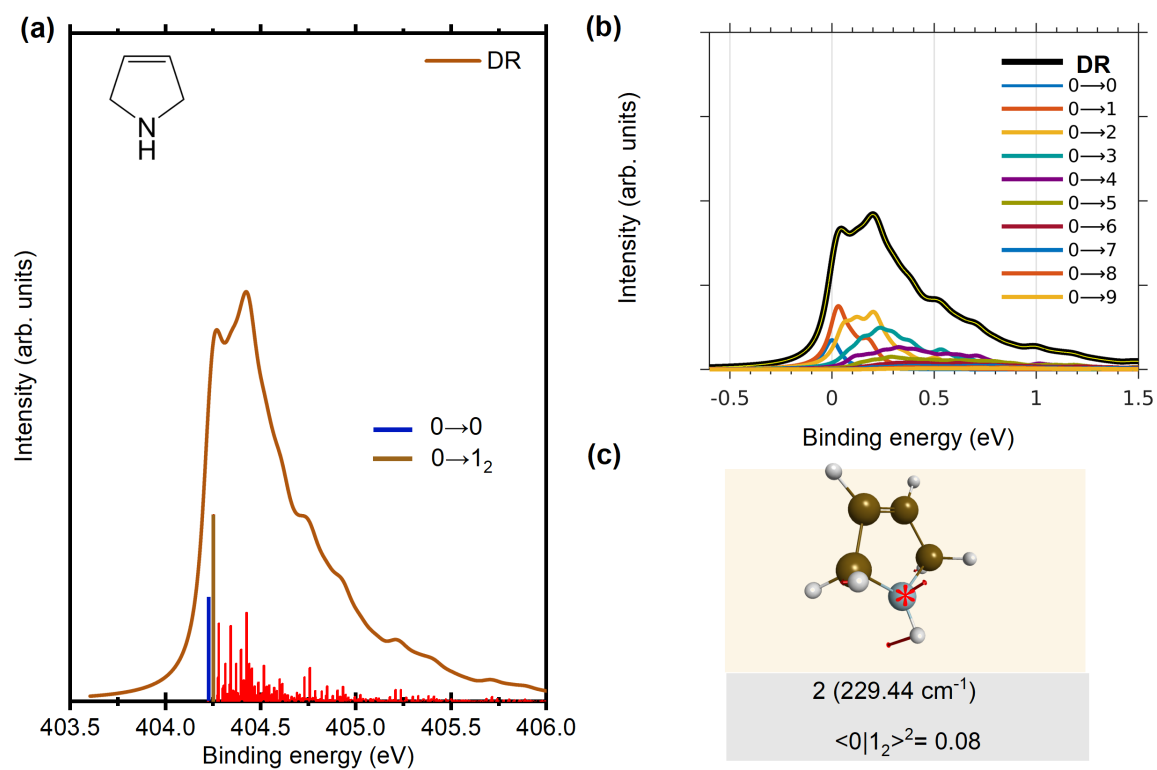

FIG. S4: The same as Fig. S2 for 3-pyrroline.

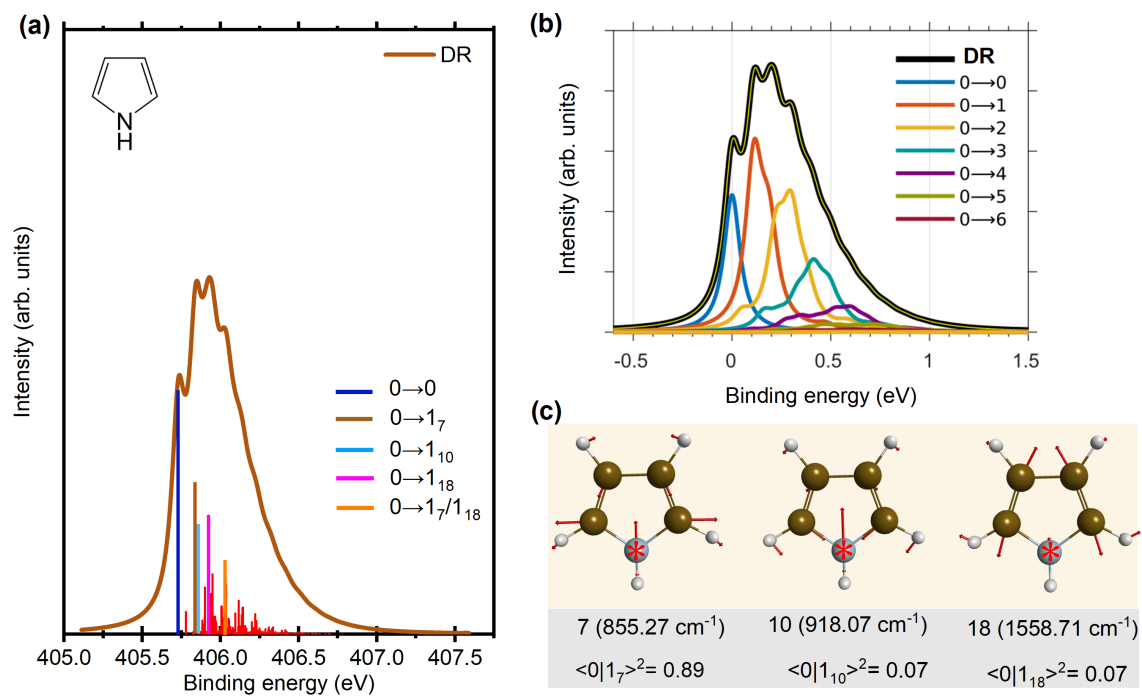

FIG. S5: The same as Fig. S2 for 1H-pyrrole.

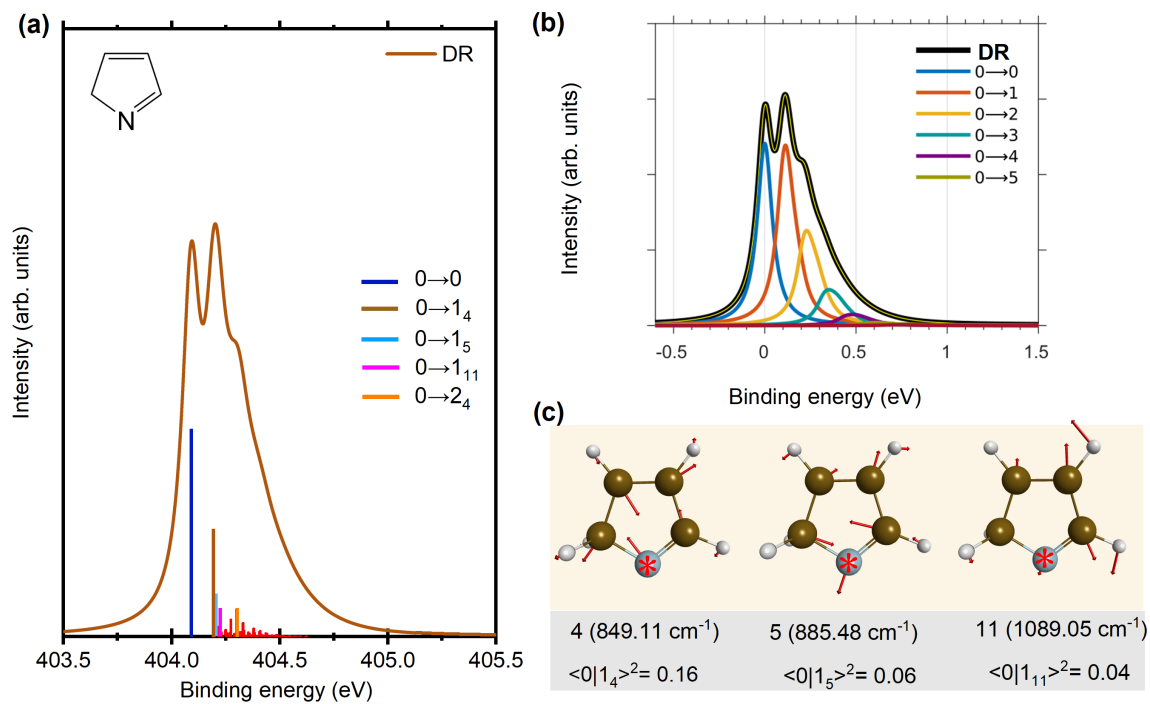

FIG. S6: The same as Fig. S2 for 2H-pyrrole.

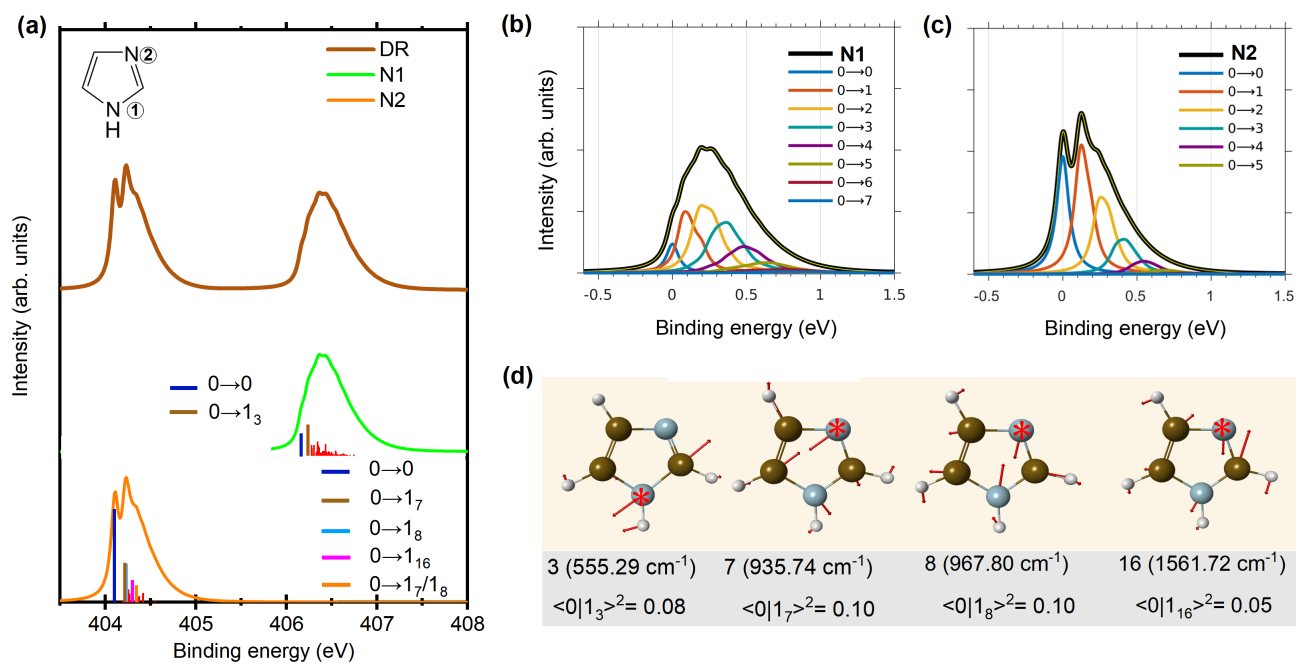

FIG. S7: (a) Simulated vibrationally-resolved N1s XPS spectrum of imidazole. (b-c) The contribution of the different 0-n transitions (until convergence) of N1 and N2. 0-0 transition energy is taken as zero. (d) Active vibrational modes are identified in the final (FCH) state. For each mode, the mode index, frequency (in parentheses), and the FC factor are shown. Asterisk denotes the core ionization center.

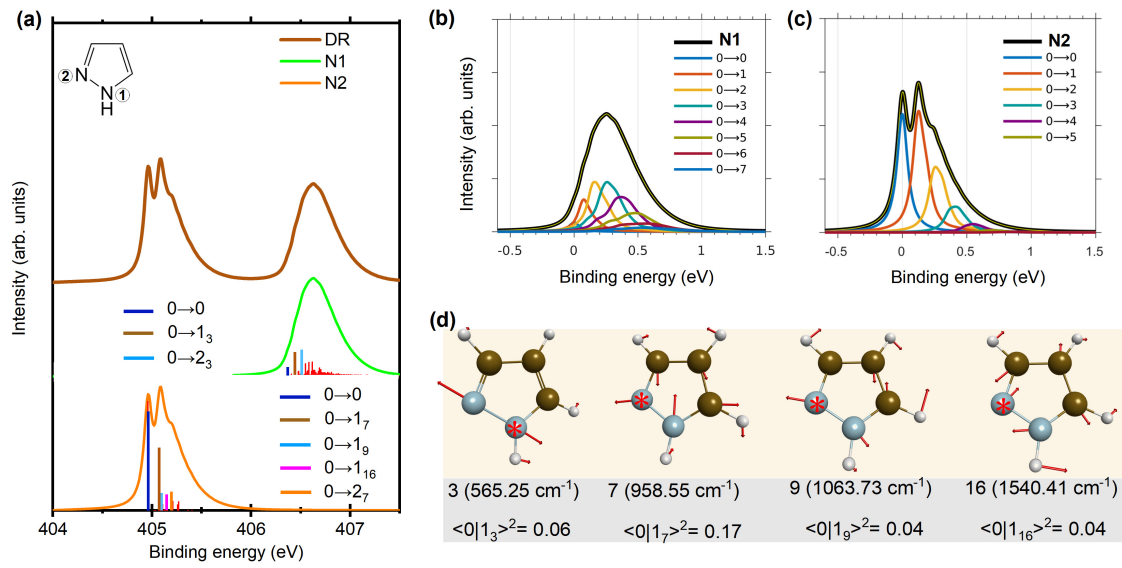

FIG. S8: The same as Fig. S7 for pyrazole.

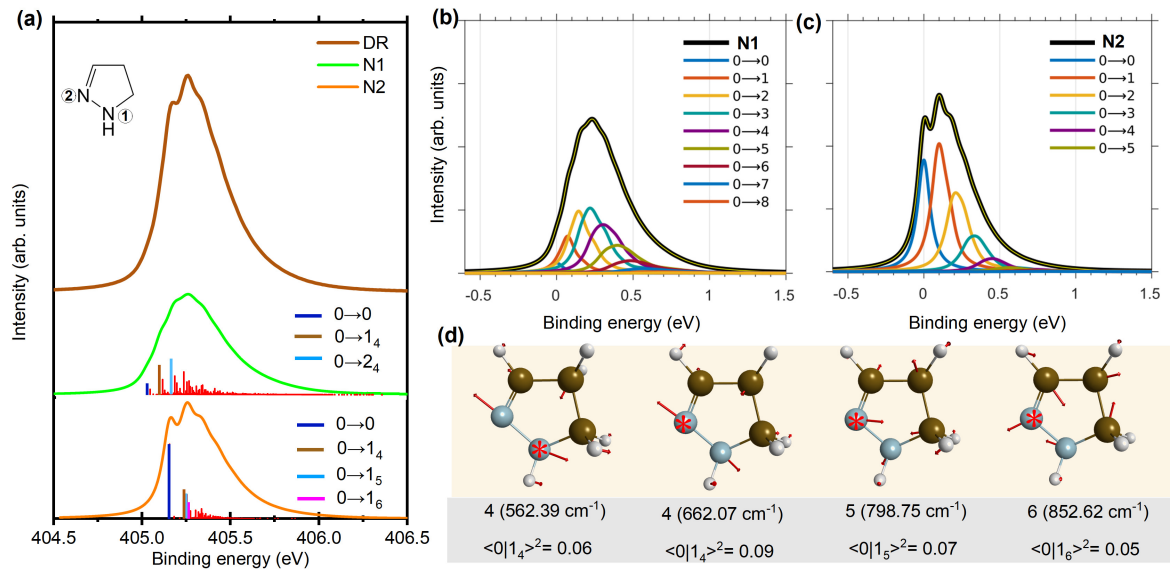

FIG. S9: The same as Fig. S7 for 2-pyrazoline.

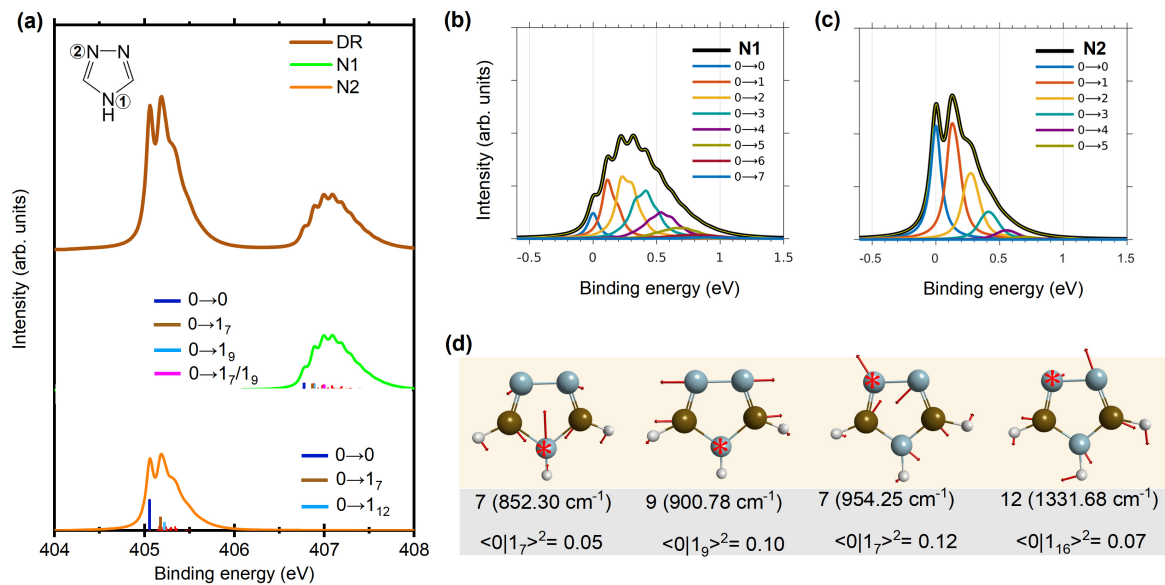

FIG. S10: The same as Fig. S7 for 1,3,4-triazole.

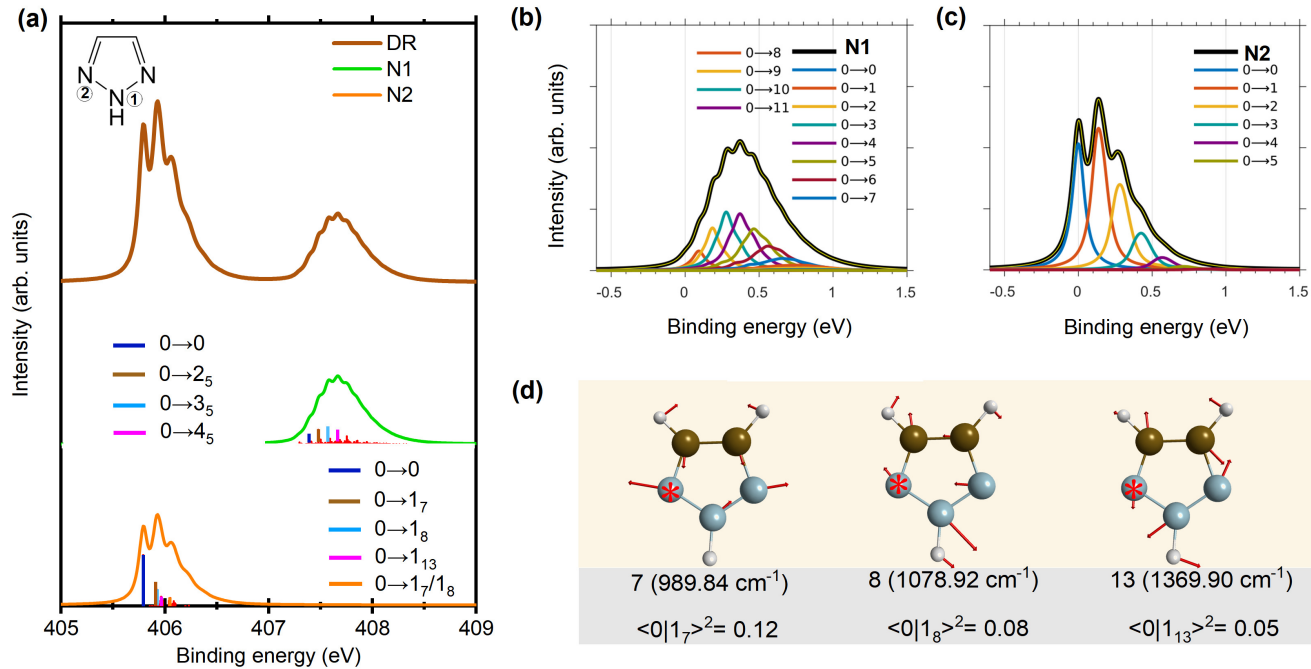

FIG. S11: The same as Fig. S7 for 1,2,5-triazole.

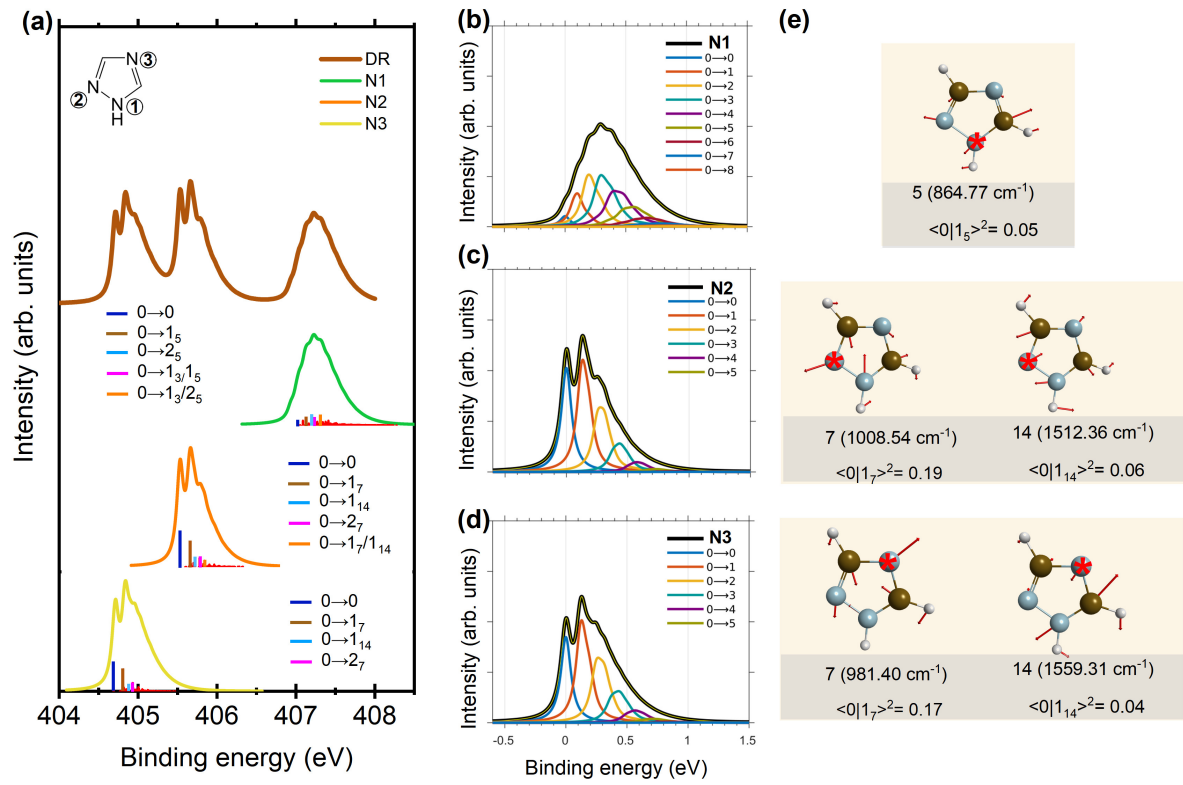

FIG. S12: (a) Simulated vibrationally-resolved N1s XPS spectrum of 1,2,4-triazole. (b-d) The contribution of the different 0- $n$  transitions (until convergence) of N1, N2, and N3. 0-0 transition energy is taken as zero. (e) Active vibrational modes are identified in the final (FCH) state. For each mode, the mode index, frequency (in parentheses), and the FC factor are shown. Asterisk denotes the core ionization center.

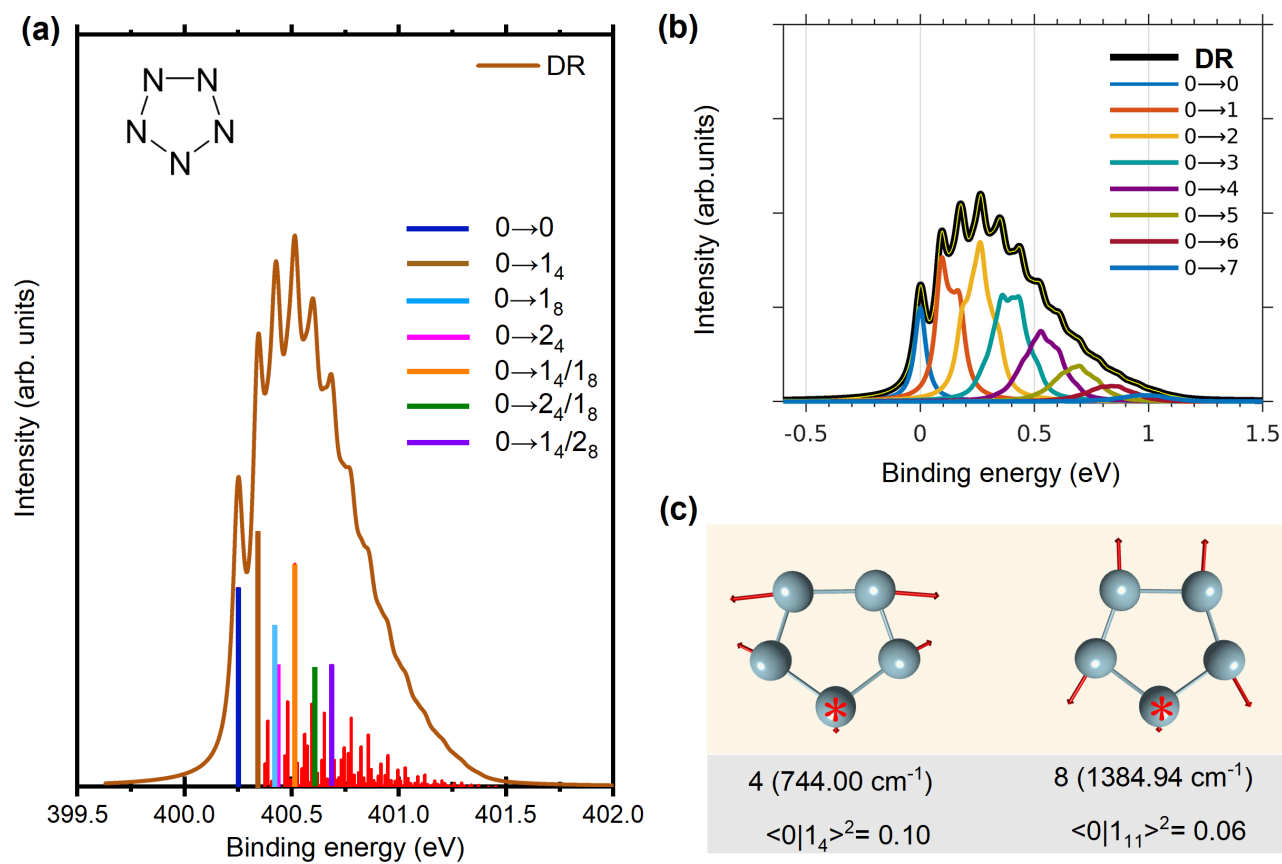

FIG. S13: The same as Fig. S2 for *cyclo-N<sub>5</sub><sup>-</sup>*.

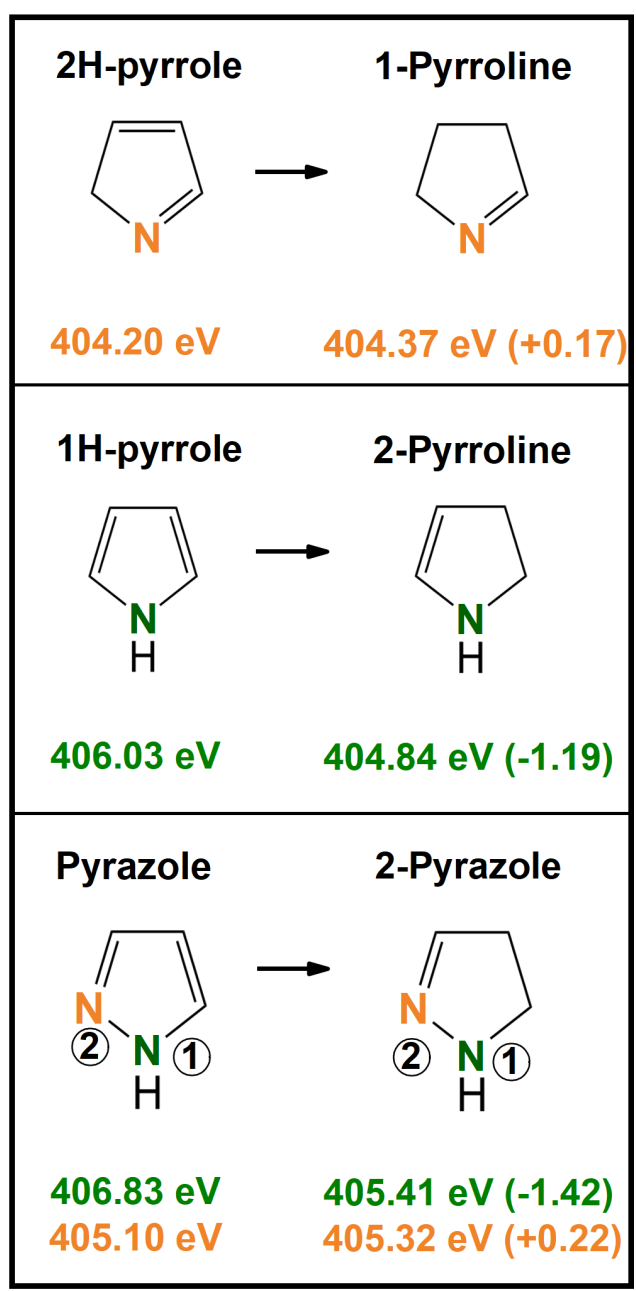

FIG. S14: Effects of hydrogenation. Comparison of computed vertical ionization potentials ( $I^{\text{vert}}$ ) for selected three pairs of molecules (two molecules in each pair differ by two hydrogen atoms).

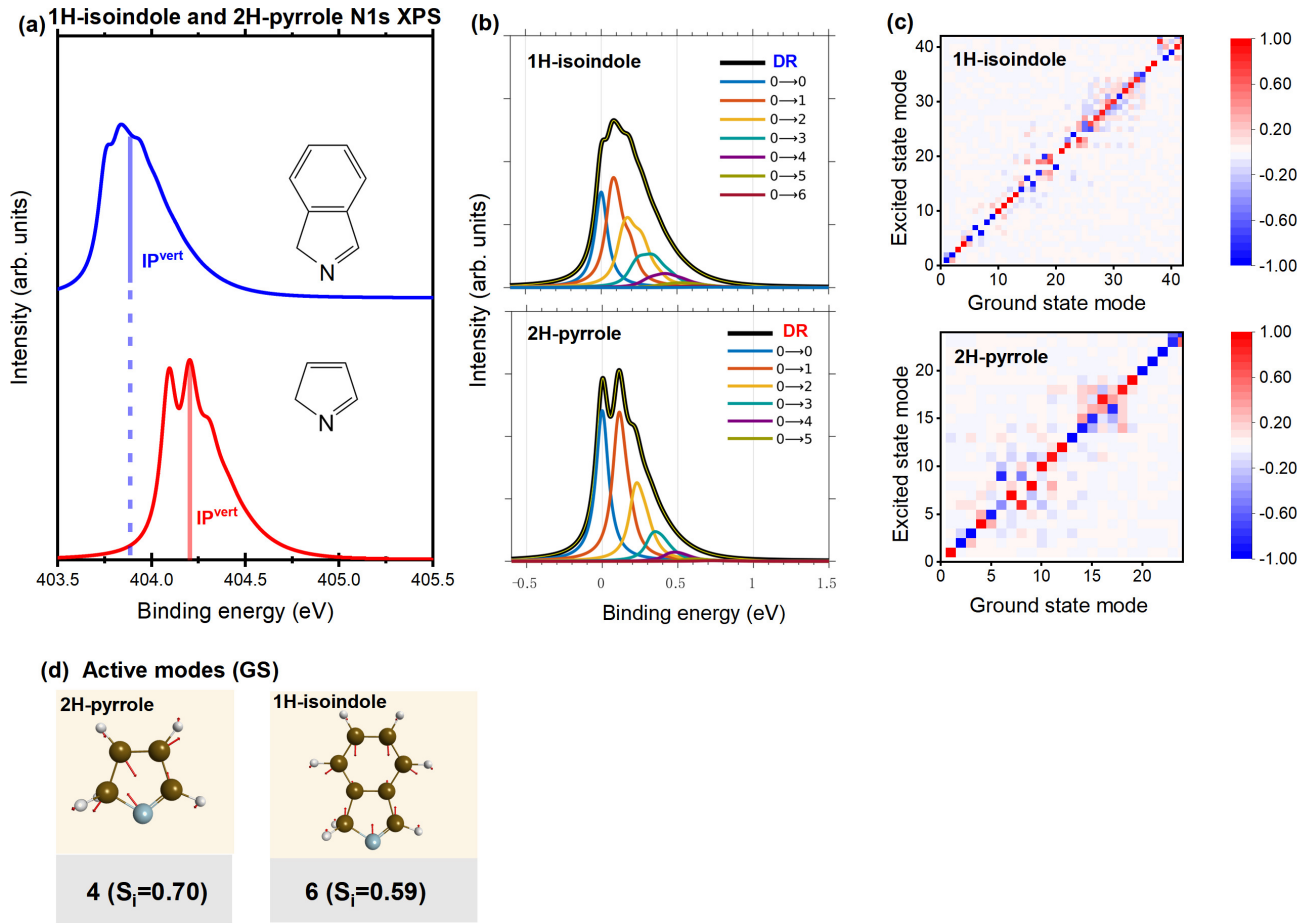

FIG. S15: A comparison of 1H-isoindole and 2H-pyrrole to see the influence of the benzene ring. (a) Computed vibrationally-resolved N1s XPS. Vertical ionization energies are indicated by vertical lines. (b) Contributions of different 0- $n$  transitions until convergence. (c) The Duschinsky matrix. (d) Active vibrational modes are identified in the ground state. For each mode, the mode index and the Huang-Rhys factor (in parentheses) are shown.

TABLE S1: Analysis of selected vibrational modes with large Huang-Rhys factors (a threshold of  $S_i \geq 0.3$  was used) for the 7 azine molecules. Vibrational frequencies  $\omega_i$  and the total vibrational reorganization energy ( $E_r$ ) of the excited (FCH) state are given.

| Molecule          | N* | $i$ | $\omega_i$ (cm <sup>-1</sup> ) | $S_i$ | $E_r$ (eV) |
|-------------------|----|-----|--------------------------------|-------|------------|
| Pyridine          | N  | 3   | 602.6                          | 0.92  | 0.14       |
| Pyrimidine        | N  | 3   | 620.2                          | 0.50  | 0.16       |
|                   |    | 4   | 674.3                          | 0.30  |            |
| Pyrazine          | N  | 3   | 592.9                          | 1.08  | 0.14       |
| Pyridazine        | N  | 3   | 615.6                          | 0.72  | 0.18       |
|                   |    | 11  | 1063.6                         | 0.40  |            |
| 1,3,5-Triazine    | N  | 4   | 683.3                          | 0.67  | 0.18       |
|                   |    | 7   | 1008.2                         | 0.35  |            |
| 1,2,4-Triazine    | N1 | 3   | 605.8                          | 0.91  | 0.18       |
|                   | N2 | 3   | 623.1                          | 0.39  | 0.20       |
|                   |    | 4   | 704.0                          | 0.50  |            |
|                   |    | 4   | 615.5                          | 0.86  |            |
|                   | N4 | 10  | 1052.9                         | 0.31  | 0.14       |
| 1,2,4,5-Tetrazine | N  | 3   | 630.0                          | 0.72  | 0.21       |
|                   |    | 7   | 963.8                          | 0.48  |            |
|                   |    | 10  | 1084.5                         | 0.35  |            |

TABLE S2: Analysis of selected vibrational modes with large Huang-Rhys factors (a threshold of  $S_i \geq 0.3$  was used) for the 17 bicyclic indole molecules. Vibrational frequencies  $\omega_i$  and the total vibrational reorganization energy ( $E_r$ ) of the excited (FCH) state are given. Amine (bold) and imine (lightface) N atoms are highlighted by different fonts.

| Molecule       | N*        | $i$ | $\omega_i$ (cm <sup>-1</sup> ) | $S_i$ | $E_r$ (eV) |
|----------------|-----------|-----|--------------------------------|-------|------------|
| Indole         | <b>N</b>  | 3   | 288.6                          | 0.40  | 0.46       |
|                |           | 27  | 1279.9                         | 0.32  |            |
|                |           | 31  | 1484.0                         | 0.56  |            |
| 3-Methylindole | <b>N</b>  | 6   | 380.2                          | 0.58  | 0.71       |
|                |           | 31  | 1293.8                         | 0.73  |            |
|                |           | 37  | 1483.7                         | 0.38  |            |
|                |           | 51  | 3799.7                         | 0.69  |            |
| 3-Formylindole | <b>N</b>  | 2   | 156.1                          | 0.36  | 0.49       |
|                |           | 8   | 419.7                          | 0.31  |            |
|                |           | 31  | 1283.6                         | 0.45  |            |
|                |           | 36  | 1477.6                         | 0.48  |            |
|                |           | 38  | 1604.1                         | 0.33  |            |
| Purine         | N1        | 6   | 585.3                          | 0.73  | 0.22       |
|                |           | 13  | 932.7                          | 0.34  |            |
|                | N2        | 10  | 788.9                          | 0.44  | 0.23       |
|                |           | 20  | 1215.9                         | 0.34  |            |
|                | N3        | 8   | 671.3                          | 0.34  | 0.23       |
|                |           | 13  | 936.2                          | 0.44  |            |
|                |           | 14  | 954.5                          | 0.42  |            |
|                | <b>N4</b> | 17  | 1017.8                         | 1.60  | 0.91       |
|                |           | 23  | 1280.8                         | 0.34  |            |
|                |           | 24  | 1339.8                         | 0.45  |            |
|                |           | 25  | 1405.0                         | 0.84  |            |
|                |           | 27  | 1574.7                         | 0.90  |            |
| Adenine        | N1        | 29  | 1701.2                         | 0.66  |            |
|                |           | 11  | 650.8                          | 0.57  |            |
|                |           | 17  | 906.3                          | 0.31  |            |
|                | N2        | 30  | 1519.3                         | 0.34  | 0.28       |
|                |           | 8   | 568.3                          | 0.40  |            |
|                |           | 18  | 965.4                          | 0.73  |            |
|                | <b>N4</b> | 21  | 1109.5                         | 0.30  | 0.25       |
|                |           | 21  | 1000.3                         | 0.97  |            |

|                             |           |    |        |      |      |
|-----------------------------|-----------|----|--------|------|------|
|                             |           | 29 | 1418.0 | 0.37 |      |
|                             |           | 31 | 1593.0 | 0.78 |      |
|                             |           | 33 | 1678.3 | 0.54 |      |
|                             | <b>N5</b> | 27 | 1359.1 | 0.33 | 0.62 |
|                             |           | 30 | 1472.2 | 0.71 |      |
|                             |           | 34 | 1720.2 | 1.04 |      |
| Benzimidazole               | <b>N1</b> | 20 | 1036.0 | 1.54 | 0.86 |
|                             |           | 24 | 1193.4 | 0.33 |      |
|                             |           | 27 | 1331.5 | 0.86 |      |
|                             |           | 29 | 1486.9 | 0.80 |      |
|                             |           | 31 | 1618.3 | 0.47 |      |
|                             | N2        | 16 | 974.2  | 0.56 | 0.20 |
| 4-Azaindole                 | <b>N1</b> | 3  | 275.5  | 0.34 | 0.49 |
|                             |           | 26 | 1300.8 | 0.31 |      |
|                             |           | 29 | 1449.6 | 0.30 |      |
|                             | N2        | 11 | 778.3  | 0.51 | 0.18 |
| 5-Azaindole                 | <b>N1</b> | 30 | 1487.6 | 0.44 | 0.42 |
|                             | N2        | 6  | 574.2  | 0.81 | 0.19 |
| 6-Azaindole                 | <b>N1</b> | 4  | 389.7  | 0.40 | 0.47 |
|                             |           | 29 | 1451.1 | 0.51 |      |
|                             | N2        | 6  | 571.6  | 0.70 | 0.19 |
| 7-Azaindole                 | <b>N1</b> | 26 | 1278.7 | 0.40 | 0.42 |
|                             |           | 29 | 1434.5 | 0.64 |      |
|                             |           | 33 | 1688.5 | 0.34 |      |
|                             | N2        | 11 | 775.9  | 0.44 | 0.18 |
| 1 <i>H</i> -isoindole       | N         | 6  | 528.1  | 0.59 | 0.16 |
| 2 <i>H</i> -indole          | N         | 13 | 873.2  | 0.84 | 0.18 |
| 3 <i>H</i> -indole          | N         | 14 | 885.6  | 0.55 | 0.16 |
| 2 <i>H</i> -isoindole       | <b>N</b>  | 21 | 1006.3 | 0.47 | 0.32 |
|                             |           | 30 | 1426.9 | 0.78 |      |
| Indolizine                  | <b>N</b>  | 12 | 715.8  | 0.41 | 0.30 |
|                             |           | 26 | 1222.5 | 0.37 |      |
| 7-Azaindazole               | <b>N1</b> | 15 | 920.8  | 0.56 | 0.76 |
|                             |           | 19 | 1059.8 | 1.82 |      |
|                             |           | 21 | 1160.7 | 0.50 |      |
|                             |           | 23 | 1206.8 | 1.03 |      |
|                             | N2        | 6  | 540.4  | 0.41 | 0.15 |
|                             |           | 15 | 945.3  | 0.34 |      |
|                             | N3        | 6  | 554.3  | 0.30 | 0.20 |
|                             |           | 10 | 774.0  | 0.42 |      |
| Pyrazolo[1,5-a]- pyrimidine | <b>N1</b> | 10 | 681.0  | 0.76 | 0.55 |
|                             |           | 13 | 827.4  | 0.52 |      |
|                             |           | 20 | 1054.1 | 0.30 |      |
|                             |           | 22 | 1135.5 | 0.49 |      |
|                             | N2        | 10 | 787.9  | 0.37 | 0.22 |
|                             | N3        | 7  | 592.3  | 0.35 | 0.19 |
|                             |           | 13 | 915.1  | 0.53 |      |

TABLE S3. Simulated vertical ( $I^{\text{vert}}$ ) and adiabatic ( $I^{\text{ad}}$ ) ionization potentials and their difference ( $\Delta I = I^{\text{vert}} - I^{\text{ad}}$ ), difference in zero-point vibrational energy ( $\Delta \epsilon_0$ ), and the total reorganization energy ( $E_r$ ) for all 35 N-heterocycle molecules studied in the three papers.

| No. | Molecule          | Core | $I^{\text{vert}}$ | $I^{\text{ad}}$ | $\Delta I$ | $\Delta \epsilon_0$ | $E_r$ |
|-----|-------------------|------|-------------------|-----------------|------------|---------------------|-------|
| 1   | 2H-pyrrole        |      | 404.20            | 404.06          | 0.14       | 0.04                | 0.14  |
| 2   | 1-Pyrroline       |      | 404.37            | 404.21          | 0.16       | 0.02                | 0.15  |
| 3   | 3-Pyrroline       |      | 404.50            | 404.21          | 0.29       | 0.02                | 0.59  |
| 4   | 2-Pyrroline       |      | 404.84            | 404.57          | 0.27       | 0.00                | 0.32  |
| 5   | 1H-Pyrrole        |      | 406.03            | 405.76          | 0.27       | -0.03               | 0.34  |
| 6   | Imidazole         | N1   | 406.59            | 406.23          | 0.36       | -0.07               | 0.58  |
|     |                   | N2   | 404.25            | 404.06          | 0.19       | 0.04                | 0.18  |
| 7   | Pyrazole          | N1   | 406.83            | 406.45          | 0.38       | -0.07               | 0.61  |
|     |                   | N2   | 405.10            | 404.94          | 0.16       | 0.02                | 0.16  |
| 8   | 2-Pyrazoline      | N1   | 405.41            | 405.06          | 0.35       | -0.03               | 0.51  |
|     |                   | N2   | 405.32            | 405.16          | 0.16       | 0.00                | 0.16  |
| 9   | 1,3,4-triazole    | N1   | 407.23            | 406.86          | 0.37       | -0.08               | 0.52  |
|     |                   | N2   | 405.21            | 405.04          | 0.17       | 0.02                | 0.17  |
| 10  | 1,2,5-triazole    | N1   | 407.87            | 407.39          | 0.48       | -0.09               | 0.63  |
|     |                   | N2   | 405.98            | 405.80          | 0.18       | -0.01               | 0.18  |
| 11  | 1,2,4-triazole    | N1   | 407.44            | 407.02          | 0.42       | 0.00                | 0.53  |
|     |                   | N2   | 405.71            | 405.53          | 0.18       | 0.02                | 0.18  |
|     |                   | N3   | 407.91            | 404.69          | 0.22       | -0.03               | 0.10  |
| 12  | Pyridine          |      | 404.50            | 404.26          | 0.24       | 0.03                | 0.14  |
| 13  | Pyrimidine        |      | 404.97            | 404.80          | 0.17       | 0.01                | 0.16  |
| 14  | Pyrazine          |      | 405.24            | 405.11          | 0.13       | 0.01                | 0.14  |
| 15  | Pyridazine        |      | 405.52            | 405.34          | 0.18       | 0.01                | 0.18  |
| 16  | 1,3,5-Triazine    |      | 405.49            | 405.30          | 0.19       | -0.01               | 0.18  |
| 17  | 1,2,4-Triazine    | N1   | 406.33            | 405.66          | 0.17       | -0.01               | 0.18  |
|     |                   | N2   | 406.01            | 405.83          | 0.18       | -0.01               | 0.20  |
|     |                   | N4   | 405.80            | 406.16          | 0.14       | -0.01               | 0.14  |
| 18  | 1,2,4,5-Tetrazine |      | 406.98            | 406.79          | 0.19       | -0.04               | 0.21  |
| 19  | Indole            |      | 405.68            | 405.29          | 0.39       | -0.02               | 0.46  |
| 20  | 3-Methylindole    |      | 405.46            | 405.11          | 0.35       | -0.01               | 0.71  |
| 21  | 3-Formylindole    |      | 406.24            | 405.90          | 0.34       | -0.05               | 0.49  |
| 22  | Adenine           | N1   | 403.91            | 403.62          | 0.29       | 0.04                | 0.29  |
|     |                   | N2   | 404.04            | 403.74          | 0.30       | 0.04                | 0.28  |
|     |                   | N3   | 404.45            | 404.19          | 0.26       | 0.03                | 0.25  |
|     |                   | N4   | 406.37            | 405.87          | 0.50       | -0.08               | 0.80  |
|     |                   | N5   | 405.47            | 405.10          | 0.37       | -0.04               | 0.62  |
| 23  | Purine            | N1   | 404.48            | 404.27          | 0.21       | 0.01                | 0.22  |
|     |                   | N2   | 404.83            | 404.60          | 0.23       | 0.00                | 0.23  |
|     |                   | N3   | 404.73            | 404.49          | 0.24       | 0.02                | 0.23  |

|    |                           |    |        |        |      |       |      |
|----|---------------------------|----|--------|--------|------|-------|------|
|    |                           | N4 | 406.75 | 406.28 | 0.47 | -0.10 | 0.91 |
| 24 | Benzimidazole             | N1 | 406.17 | 405.76 | 0.41 | -0.08 | 0.86 |
|    |                           | N2 | 404.00 | 403.78 | 0.22 | 0.04  | 0.20 |
| 25 | 4-Azaindole               | N1 | 405.98 | 405.68 | 0.30 | -0.03 | 0.49 |
|    |                           | N2 | 403.81 | 403.63 | 0.18 | 0.04  | 0.18 |
| 26 | 5-Azaindole               | N1 | 406.07 | 405.77 | 0.30 | -0.04 | 0.42 |
|    |                           | N2 | 403.76 | 403.57 | 0.19 | 0.05  | 0.19 |
| 27 | 6-Azaindole               | N1 | 406.07 | 405.77 | 0.30 | -0.04 | 0.47 |
|    |                           | N2 | 403.77 | 403.60 | 0.17 | 0.04  | 0.19 |
| 28 | 7-Azaindole               | N1 | 405.82 | 405.48 | 0.34 | -0.04 | 0.42 |
|    |                           | N2 | 404.10 | 403.92 | 0.18 | 0.03  | 0.18 |
| 29 | 1H-isoindole              |    | 403.88 | 403.71 | 0.17 | 0.04  | 0.16 |
| 30 | 2H-indole                 |    | 403.31 | 403.13 | 0.18 | 0.05  | 0.18 |
| 31 | 3H-indole                 |    | 404.52 | 404.36 | 0.16 | 0.00  | 0.16 |
| 32 | 2H-isoindole              |    | 406.07 | 405.80 | 0.27 | -0.04 | 0.32 |
| 33 | Indoline                  |    | 406.18 | 405.92 | 0.26 | -0.03 | 0.30 |
| 34 | 7-Azaindazole             | N1 | 406.43 | 405.97 | 0.46 | -0.07 | 0.76 |
|    |                           | N2 | 405.19 | 405.03 | 0.16 | 0.00  | 0.15 |
|    |                           | N3 | 404.51 | 404.31 | 0.20 | 0.02  | 0.20 |
| 35 | Pyrazolo[1,5-a]pyrimidine | N1 | 407.15 | 406.75 | 0.40 | -0.07 | 0.55 |
|    |                           | N2 | 404.66 | 404.45 | 0.21 | 0.01  | 0.22 |
|    |                           | N3 | 404.80 | 404.60 | 0.20 | 0.02  | 0.19 |

TABLE S4. Superposition of the optimized ground state and the N1s ionized state geometries (*leftmost*) and the ground-state active vibrational modes (*right*) for all 35 molecules studied in three papers of this series. The core ionization center is illustrated with a black circle. Active modes were filtered according to a threshold of HRFs ( $S_i \geq 0.3$ ). Amine (bold) and imine (lightface) N atoms are distinguished in different fonts. For each mode, the mode index and the HRF (in parentheses) are specified. 35 molecules include 11 monocyclic compounds with five-membered rings, 7 monocyclic compounds with six-membered rings, and 17 bicyclic compounds consisting of fused five- and six-membered rings.

**Part 1: 11 Monocyclic Compounds with Five-Membered Rings**

|                 |                                                                                                          |                                                                                                          |                                                                                                          |  |  |
|-----------------|----------------------------------------------------------------------------------------------------------|----------------------------------------------------------------------------------------------------------|----------------------------------------------------------------------------------------------------------|--|--|
| 2H-pyrrole (N)  | 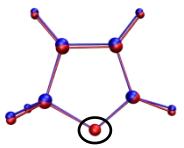<br>4 ( $S_i=0.70$ )    |                                                                                                          |                                                                                                          |  |  |
| 1-Pyrroline (N) | 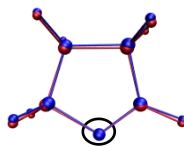<br>5 ( $S_i=0.41$ )   |                                                                                                          |                                                                                                          |  |  |
| 3-Pyrroline (N) | 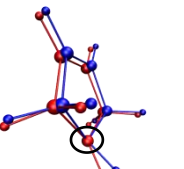<br>3 ( $S_i=1.39$ )  | 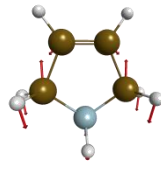<br>19 ( $S_i=0.85$ ) | 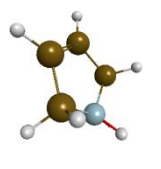<br>30 ( $S_i=0.50$ ) |  |  |
| 2-Pyrroline (N) | 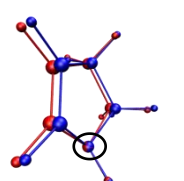<br>1 ( $S_i=0.65$ )  | 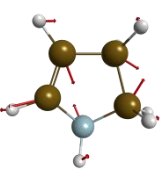<br>19 ( $S_i=0.33$ ) | 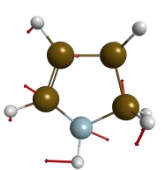<br>30 ( $S_i=0.36$ ) |  |  |
| 1H-pyrrole (N)  | 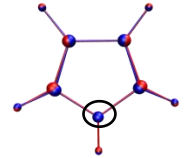<br>12 ( $S_i=0.40$ ) | 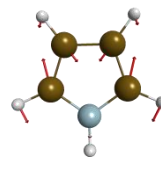<br>18 ( $S_i=1.03$ ) |                                                                                                          |  |  |

|                   |                                                                                     |                                                                                                         |                                                                                                         |                                                                                                           |                                                                                                            |                                                                                                          |
|-------------------|-------------------------------------------------------------------------------------|---------------------------------------------------------------------------------------------------------|---------------------------------------------------------------------------------------------------------|-----------------------------------------------------------------------------------------------------------|------------------------------------------------------------------------------------------------------------|----------------------------------------------------------------------------------------------------------|
| Imidazole (N1)    | 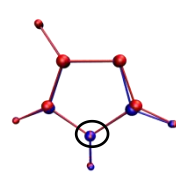   | 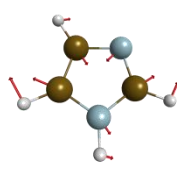<br>9 ( $S_i=0.36$ )   | 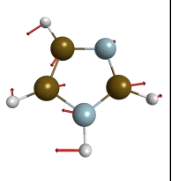<br>10 ( $S_i=0.31$ )  | 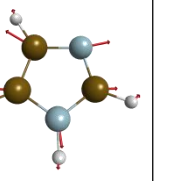<br>12 ( $S_i=0.58$ )   | 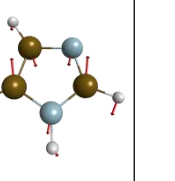<br>16 ( $S_i=1.73$ )   |                                                                                                          |
| Imidazole (N2)    | 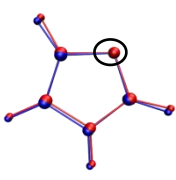   | 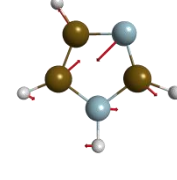<br>7 ( $S_i=0.72$ )   |                                                                                                         |                                                                                                           |                                                                                                            |                                                                                                          |
| Pyrazole (N1)     | 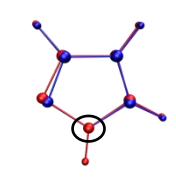   | 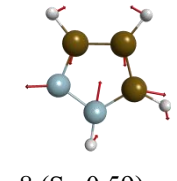<br>8 ( $S_i=0.59$ )   | 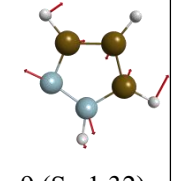<br>9 ( $S_i=1.32$ )   | 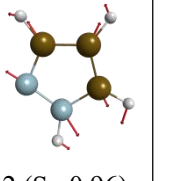<br>12 ( $S_i=0.96$ )   | 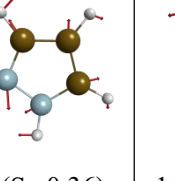<br>13 ( $S_i=0.36$ )   | 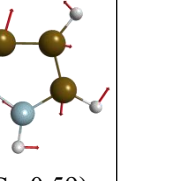<br>14 ( $S_i=0.59$ ) |
| Pyrazole (N2)     | 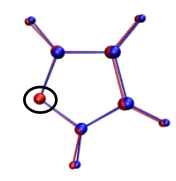 | 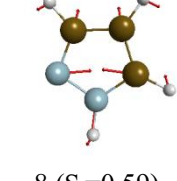<br>8 ( $S_i=0.59$ ) |                                                                                                         |                                                                                                           |                                                                                                            |                                                                                                          |
| 2-Pyrazoline (N1) | 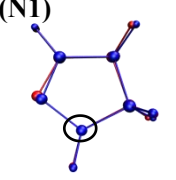 | 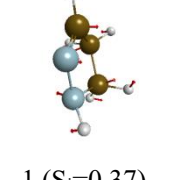<br>1 ( $S_i=0.37$ ) | 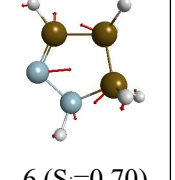<br>6 ( $S_i=0.70$ ) | 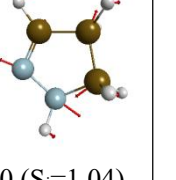<br>10 ( $S_i=1.04$ ) | 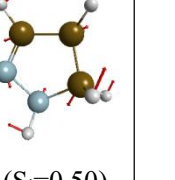<br>17 ( $S_i=0.50$ ) |                                                                                                          |
| 2-Pyrazoline (N2) | 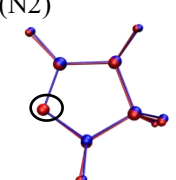 | 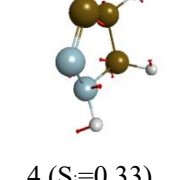<br>4 ( $S_i=0.33$ ) | 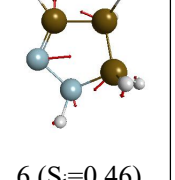<br>6 ( $S_i=0.46$ ) |                                                                                                           |                                                                                                            |                                                                                                          |

|                        |                                                                                     |                                                                                                         |                                                                                                         |                                                                                                          |                                                                                                            |                                                                                                            |
|------------------------|-------------------------------------------------------------------------------------|---------------------------------------------------------------------------------------------------------|---------------------------------------------------------------------------------------------------------|----------------------------------------------------------------------------------------------------------|------------------------------------------------------------------------------------------------------------|------------------------------------------------------------------------------------------------------------|
| 1,3,4-Triazole<br>(N1) | 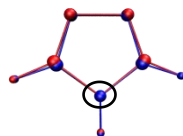   | 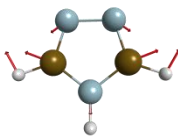<br>10 ( $S_i=0.82$ )  | 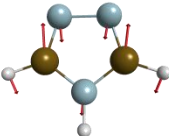<br>15 ( $S_i=1.76$ )  |                                                                                                          |                                                                                                            |                                                                                                            |
| 1,3,4-Triazole<br>(N2) | 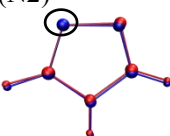   | 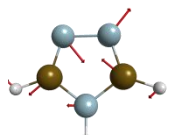<br>6 ( $S_i=0.56$ )   | 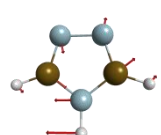<br>15 ( $S_i=0.30$ )  |                                                                                                          |                                                                                                            |                                                                                                            |
| 1,2,5-Triazole<br>(N1) | 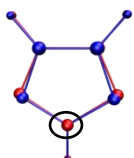   | 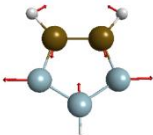<br>7 ( $S_i=1.95$ )   | 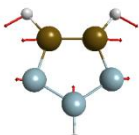<br>8 ( $S_i=0.45$ )   | 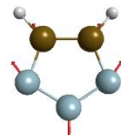<br>10 ( $S_i=1.90$ )   | 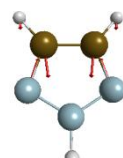<br>12 ( $S_i=0.42$ )   |                                                                                                            |
| 1,2,5-Triazole<br>(N2) | 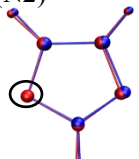 | 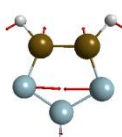<br>7 ( $S_i=0.70$ ) |                                                                                                         |                                                                                                          |                                                                                                            |                                                                                                            |
| 1,2,4-Triazole<br>(N1) | 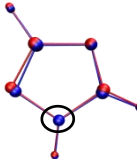 | 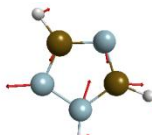<br>7 ( $S_i=0.72$ ) | 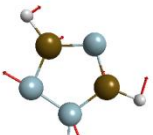<br>8 ( $S_i=1.27$ ) | 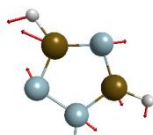<br>10 ( $S_i=0.50$ ) | 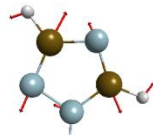<br>12 ( $S_i=0.39$ ) | 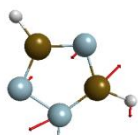<br>12 ( $S_i=0.32$ ) |
| 1,2,4-Triazole<br>(N2) | 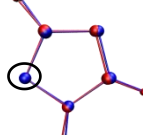 | 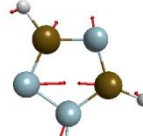<br>7 ( $S_i=0.59$ ) |                                                                                                         |                                                                                                          |                                                                                                            |                                                                                                            |

|                        |                                                                                   |                                                                                   |  |  |  |
|------------------------|-----------------------------------------------------------------------------------|-----------------------------------------------------------------------------------|--|--|--|
| 1,2,4-Triazole<br>(N3) | 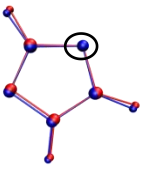 | 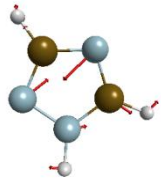 |  |  |  |
|                        |                                                                                   | 6 ( $S_i=0.84$ )                                                                  |  |  |  |

**Part 2: 7 Monocyclic Compounds with Six-Membered Rings**

|                    |                                                                                     |                                                                                     |                                                                                     |  |  |
|--------------------|-------------------------------------------------------------------------------------|-------------------------------------------------------------------------------------|-------------------------------------------------------------------------------------|--|--|
| Pyridine (N)       | 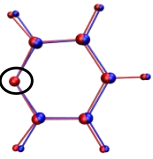   | 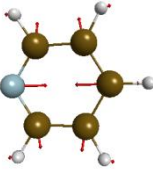   |                                                                                     |  |  |
|                    |                                                                                     | 3 ( $S_i=0.92$ )                                                                    |                                                                                     |  |  |
| Pyrimidine (N)     | 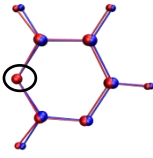  | 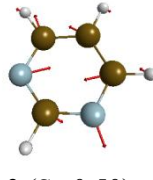  | 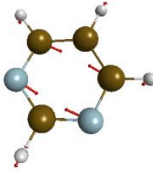  |  |  |
|                    |                                                                                     | 3 ( $S_i=0.50$ )                                                                    | 4 ( $S_i=0.30$ )                                                                    |  |  |
| Pyrazine (N)       | 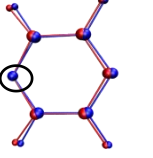 | 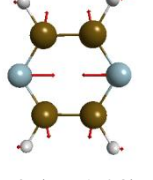 |                                                                                     |  |  |
|                    |                                                                                     | 3 ( $S_i=1.08$ )                                                                    |                                                                                     |  |  |
| Pyridazine (N)     | 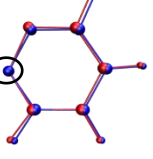 | 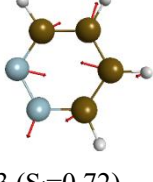 | 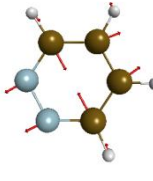 |  |  |
|                    |                                                                                     | 3 ( $S_i=0.72$ )                                                                    | 11 ( $S_i=0.40$ )                                                                   |  |  |
| 1,3,5-Triazine (N) | 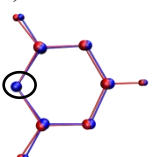 | 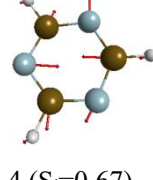 | 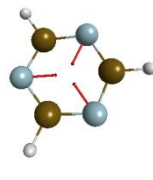 |  |  |
|                    |                                                                                     | 4 ( $S_i=0.67$ )                                                                    | 11 ( $S_i=0.35$ )                                                                   |  |  |

|                          |                                                                                     |                                                                                     |                                                                                     |                                                                                     |  |  |
|--------------------------|-------------------------------------------------------------------------------------|-------------------------------------------------------------------------------------|-------------------------------------------------------------------------------------|-------------------------------------------------------------------------------------|--|--|
| 1,2,4-Triazine<br>(N1)   | 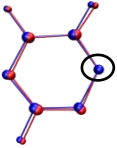   | 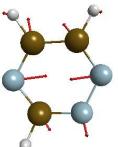   |                                                                                     |                                                                                     |  |  |
|                          |                                                                                     | 3 ( $S_i=0.91$ )                                                                    |                                                                                     |                                                                                     |  |  |
| 1,2,4-Triazine<br>(N2)   | 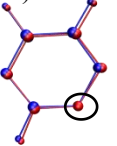   | 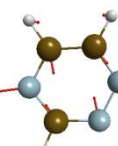   | 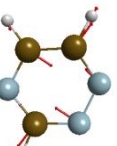   |                                                                                     |  |  |
|                          |                                                                                     | 3 ( $S_i=0.39$ )                                                                    | 4 ( $S_i=0.91$ )                                                                    |                                                                                     |  |  |
| 1,2,4-Triazine<br>(N4)   | 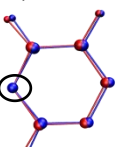   | 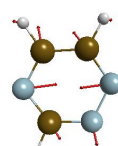   | 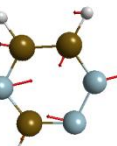   |                                                                                     |  |  |
|                          |                                                                                     | 3 ( $S_i=0.39$ )                                                                    | 10 ( $S_i=0.31$ )                                                                   |                                                                                     |  |  |
| 1,2,4,5-Tetrazine<br>(N) | 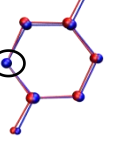 | 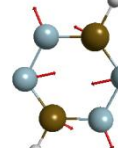 | 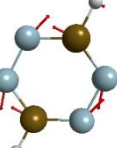 | 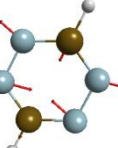 |  |  |
|                          |                                                                                     | 3 ( $S_i=0.72$ )                                                                    | 7 ( $S_i=0.48$ )                                                                    | 10 ( $S_i=0.35$ )                                                                   |  |  |

### Part 3: 17 Bicyclic Compounds Consisting of Fused Five- and Six-Membered rings

|                       |                                                                                     |                                                                                     |                                                                                     |                                                                                     |                                                                                      |  |  |
|-----------------------|-------------------------------------------------------------------------------------|-------------------------------------------------------------------------------------|-------------------------------------------------------------------------------------|-------------------------------------------------------------------------------------|--------------------------------------------------------------------------------------|--|--|
| Indole (N)            | 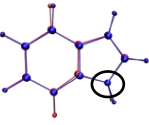 | 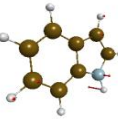 | 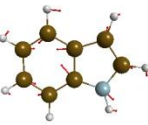 | 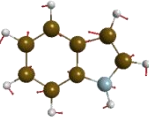 |                                                                                      |  |  |
|                       |                                                                                     | 3 ( $S_i=0.40$ )                                                                    | 27 ( $S_i=0.32$ )                                                                   | 31 ( $S_i=0.56$ )                                                                   |                                                                                      |  |  |
| 3-Methylindole<br>(N) | 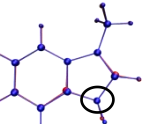 | 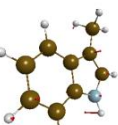 | 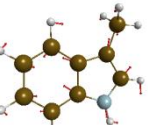 | 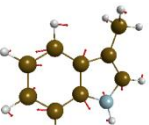 | 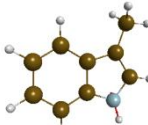 |  |  |
|                       |                                                                                     | 6 ( $S_i=0.58$ )                                                                    | 31 ( $S_i=0.73$ )                                                                   | 37 ( $S_i=0.38$ )                                                                   | 51 ( $S_i=0.69$ )                                                                    |  |  |

|                                                                                                         |                                                                                                          |                                                                                                          |                                                                                                          |                                                                                                           |                                                                                                            |                                                                                                            |
|---------------------------------------------------------------------------------------------------------|----------------------------------------------------------------------------------------------------------|----------------------------------------------------------------------------------------------------------|----------------------------------------------------------------------------------------------------------|-----------------------------------------------------------------------------------------------------------|------------------------------------------------------------------------------------------------------------|------------------------------------------------------------------------------------------------------------|
| 3-Formylindole<br>(N) 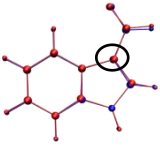 | 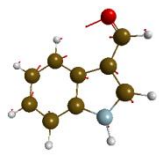<br>2 ( $S_i=0.36$ )    | 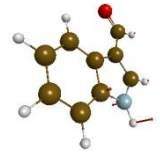<br>8 ( $S_i=0.31$ )    | 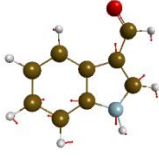<br>31 ( $S_i=0.45$ )   | 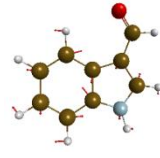<br>36 ( $S_i=0.48$ )   | 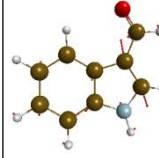<br>38 ( $S_i=0.33$ )   |                                                                                                            |
| Purine (N1) 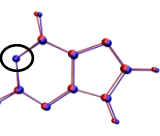           | 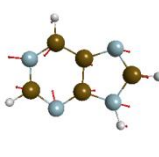<br>6 ( $S_i=0.73$ )    | 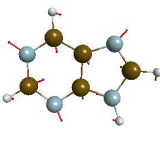<br>13 ( $S_i=0.34$ )   |                                                                                                          |                                                                                                           |                                                                                                            |                                                                                                            |
| Purine (N2) 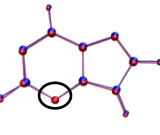           | 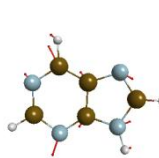<br>10 ( $S_i=0.44$ )   | 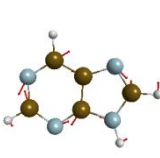<br>20 ( $S_i=0.34$ )   |                                                                                                          |                                                                                                           |                                                                                                            |                                                                                                            |
| Purine (N3) 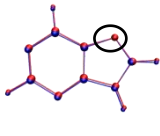         | 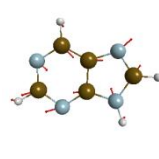<br>8 ( $S_i=0.34$ )  | 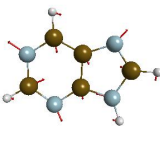<br>13 ( $S_i=0.44$ ) | 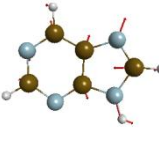<br>14 ( $S_i=0.42$ ) |                                                                                                           |                                                                                                            |                                                                                                            |
| Purine (N4) 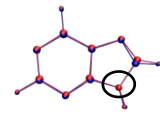         | 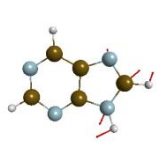<br>17 ( $S_i=1.60$ ) | 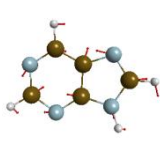<br>23 ( $S_i=0.34$ ) | 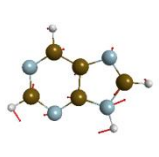<br>24 ( $S_i=0.45$ ) | 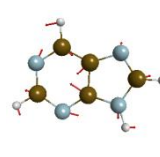<br>25 ( $S_i=0.84$ ) | 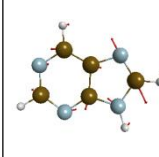<br>27 ( $S_i=0.90$ ) | 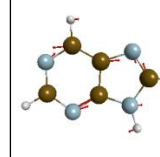<br>29 ( $S_i=0.66$ ) |
| Adenine (N1) 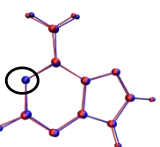        | 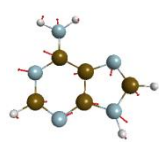<br>11 ( $S_i=0.57$ ) | 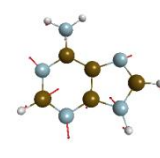<br>17 ( $S_i=0.31$ ) | 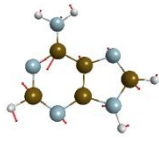<br>30 ( $S_i=0.34$ ) |                                                                                                           |                                                                                                            |                                                                                                            |

|                    |                                                                                                          |                                                                                                          |                                                                                                          |                                                                                                           |                                                                                                            |  |
|--------------------|----------------------------------------------------------------------------------------------------------|----------------------------------------------------------------------------------------------------------|----------------------------------------------------------------------------------------------------------|-----------------------------------------------------------------------------------------------------------|------------------------------------------------------------------------------------------------------------|--|
| Adenine (N2)       | 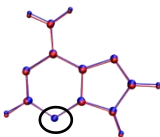<br>8 ( $S_i=0.40$ )    |                                                                                                          |                                                                                                          |                                                                                                           |                                                                                                            |  |
| Adenine (N3)       | 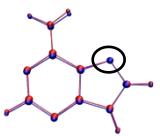<br>18 ( $S_i=0.73$ )   | 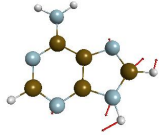<br>21 ( $S_i=0.30$ )   |                                                                                                          |                                                                                                           |                                                                                                            |  |
| Adenine (N4)       | 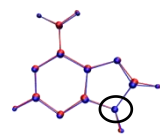<br>21 ( $S_i=0.97$ )   | 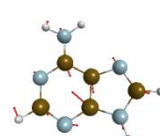<br>29 ( $S_i=0.37$ )   | 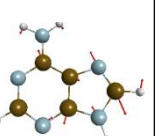<br>31 ( $S_i=0.78$ )   | 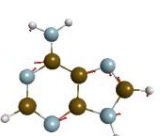<br>33 ( $S_i=0.54$ )   |                                                                                                            |  |
| Adenine (N5)       | 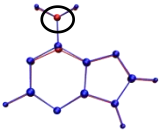<br>27 ( $S_i=0.33$ ) | 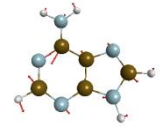<br>30 ( $S_i=0.71$ ) | 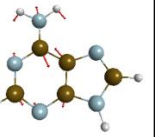<br>34 ( $S_i=1.04$ ) |                                                                                                           |                                                                                                            |  |
| Benzimidazole (N1) | 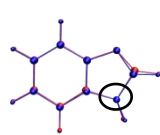<br>20 ( $S_i=1.54$ ) | 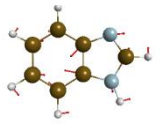<br>24 ( $S_i=0.33$ ) | 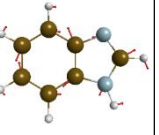<br>27 ( $S_i=0.86$ ) | 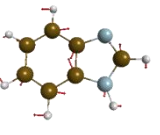<br>29 ( $S_i=0.80$ ) | 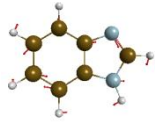<br>31 ( $S_i=0.47$ ) |  |
| Benzimidazole (N2) | 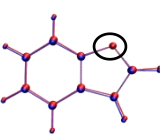<br>16 ( $S_i=0.56$ ) |                                                                                                          |                                                                                                          |                                                                                                           |                                                                                                            |  |

|                                                                                                            |                                                                                                         |                                                                                                          |                                                                                                        |  |  |  |
|------------------------------------------------------------------------------------------------------------|---------------------------------------------------------------------------------------------------------|----------------------------------------------------------------------------------------------------------|--------------------------------------------------------------------------------------------------------|--|--|--|
| 4-Azaindole<br>(N1)<br>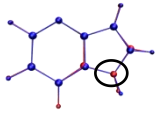   | 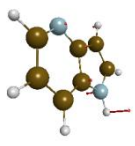<br>3 ( $S_i=0.34$ )   | 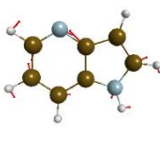<br>26 ( $S_i=0.31$ )   | 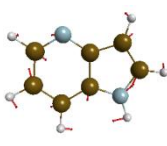<br>29 ( $S_i=0.30$ ) |  |  |  |
| 4-Azaindole<br>(N2)<br>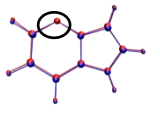   | 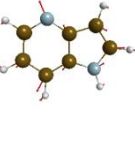<br>11 ( $S_i=0.51$ )  |                                                                                                          |                                                                                                        |  |  |  |
| 5-Azaindole<br>(N1)<br>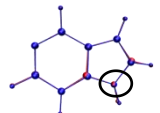   | 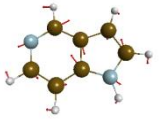<br>30 ( $S_i=0.44$ )  |                                                                                                          |                                                                                                        |  |  |  |
| 5-Azaindole<br>(N2)<br>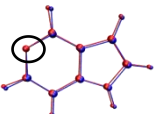 | 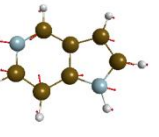<br>6 ( $S_i=0.81$ ) |                                                                                                          |                                                                                                        |  |  |  |
| 6-Azaindole<br>(N1)<br>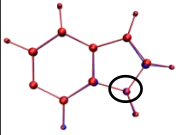 | 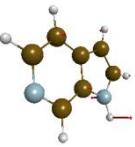<br>4 ( $S_i=0.40$ ) | 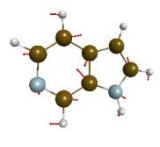<br>29 ( $S_i=0.51$ ) |                                                                                                        |  |  |  |
| 6-Azaindole<br>(N2)<br>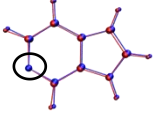 | 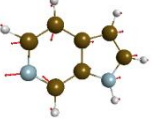<br>6 ( $S_i=0.70$ ) |                                                                                                          |                                                                                                        |  |  |  |

|                                                                                                         |                                                                                                          |                                                                                                          |                                                                                                        |  |  |  |
|---------------------------------------------------------------------------------------------------------|----------------------------------------------------------------------------------------------------------|----------------------------------------------------------------------------------------------------------|--------------------------------------------------------------------------------------------------------|--|--|--|
| 7-Azaindole<br>(N1) 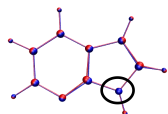   | 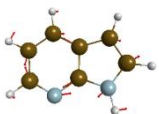<br>26 ( $S_i=0.40$ )   | 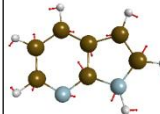<br>29 ( $S_i=0.64$ )   | 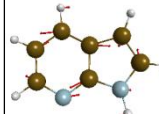<br>33 ( $S_i=0.34$ ) |  |  |  |
| 7-Azaindole<br>(N2) 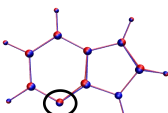   | 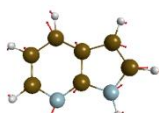<br>11 ( $S_i=0.44$ )   |                                                                                                          |                                                                                                        |  |  |  |
| 1H-isoindole<br>(N) 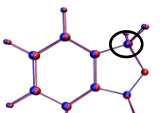   | 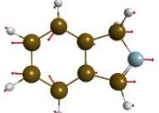<br>6 ( $S_i=0.59$ )    |                                                                                                          |                                                                                                        |  |  |  |
| 2H-indole (N) 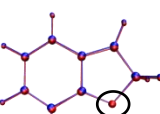       | 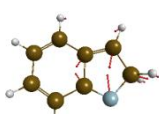<br>13 ( $S_i=0.84$ ) |                                                                                                          |                                                                                                        |  |  |  |
| 3H-indole (N) 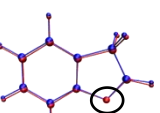       | 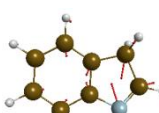<br>14 ( $S_i=0.55$ ) |                                                                                                          |                                                                                                        |  |  |  |
| 2H-isoindole<br>(N) 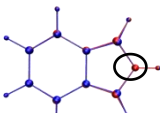 | 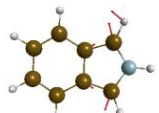<br>21 ( $S_i=0.47$ ) | 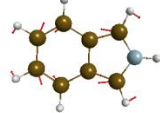<br>30 ( $S_i=0.78$ ) |                                                                                                        |  |  |  |

|                                                                                                                            |                                                                                                          |                                                                                                          |                                                                                                          |                                                                                                           |  |  |
|----------------------------------------------------------------------------------------------------------------------------|----------------------------------------------------------------------------------------------------------|----------------------------------------------------------------------------------------------------------|----------------------------------------------------------------------------------------------------------|-----------------------------------------------------------------------------------------------------------|--|--|
| Indolizine (N)<br>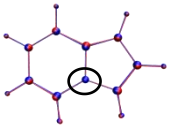                        | 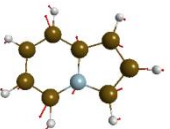<br>12 ( $S_i=0.41$ )   | 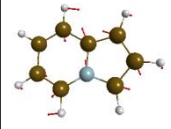<br>26 ( $S_i=0.37$ )   |                                                                                                          |                                                                                                           |  |  |
| 7-Azaindazole (N1)<br>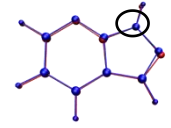                    | 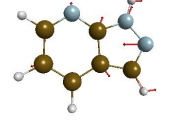<br>15 ( $S_i=0.56$ )   | 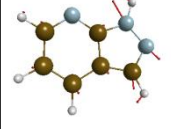<br>19 ( $S_i=1.82$ )   | 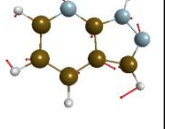<br>21 ( $S_i=0.50$ )   | 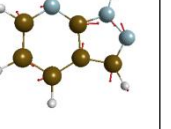<br>23 ( $S_i=1.03$ )   |  |  |
| 7-Azaindazole (N2)<br>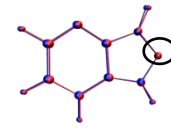                    | 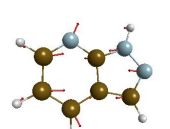<br>6 ( $S_i=0.41$ )    | 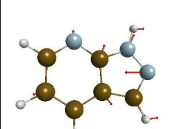<br>15 ( $S_i=0.34$ )   |                                                                                                          |                                                                                                           |  |  |
| 7-Azaindazole (N3)<br>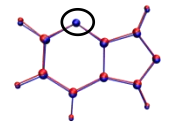                  | 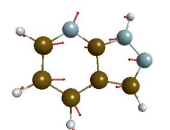<br>6 ( $S_i=0.30$ )  | 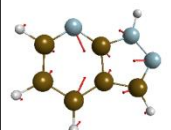<br>10 ( $S_i=0.42$ ) |                                                                                                          |                                                                                                           |  |  |
| Pyrazolo[1,5-a]<br>-pyrimidine (N1)<br>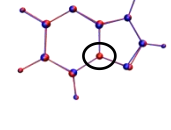 | 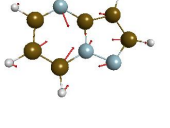<br>10 ( $S_i=0.76$ ) | 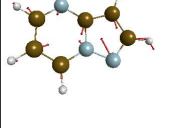<br>13 ( $S_i=0.52$ ) | 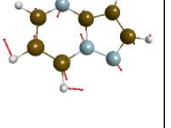<br>20 ( $S_i=0.30$ ) | 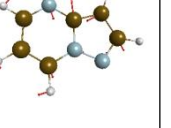<br>22 ( $S_i=0.49$ ) |  |  |
| Pyrazolo[1,5-a]<br>-pyrimidine (N2)<br>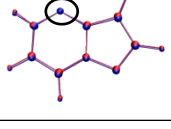 | 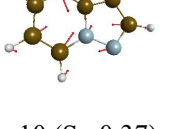<br>10 ( $S_i=0.37$ ) |                                                                                                          |                                                                                                          |                                                                                                           |  |  |

|                                                                                                                                   |                                                                                                                    |                                                                                                                     |  |  |  |  |
|-----------------------------------------------------------------------------------------------------------------------------------|--------------------------------------------------------------------------------------------------------------------|---------------------------------------------------------------------------------------------------------------------|--|--|--|--|
| <p>Pyrazolo[1,5-a]<br/>-pyrimidine<br/>(N3)</p> 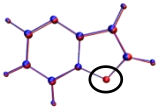 | 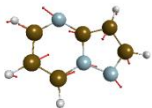 <p>7 (<math>S_i=0.35</math>)</p> | 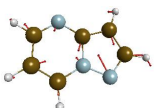 <p>13 (<math>S_i=0.53</math>)</p> |  |  |  |  |
|-----------------------------------------------------------------------------------------------------------------------------------|--------------------------------------------------------------------------------------------------------------------|---------------------------------------------------------------------------------------------------------------------|--|--|--|--|
